# Supplementary material for: Computational Role of Collective Tunneling in a Quantum Annealer
Source: arXiv:1411.4036 source file (2015-02-19)
Supplement: Supplementary file 1 [file tunneling_renormalization_appendix.tex]

\section{Lamb shift}
The imaginary part or Lamb shift of the bath coupling $\Gamma(\omega)$ has the form
\begin{align}
  S(\omega) &= \mathcal P \int_{-\infty}^{\infty}
  \frac{d\omega^{\prime }}{2\pi} \frac{\gamma(\omega^{\prime })}{\omega - \omega^{\prime }}\;.
\end{align}
For an Ohmic bath with high frequency cutoff $\omega_c$ we can choose the boundaries for
the integral to be $[-\kappa T, \kappa \omega_c]$, for some big enough
constant $\kappa$. We can treat the singularity in the calculation of
the Cauchy's principal value by writing
\begin{align}
     \mathcal P \int_{-\kappa T}^{\kappa \omega_c}
  \frac{d\omega^{\prime }}{2\pi} \frac{\gamma(\omega^{\prime })}{\omega - \omega^{\prime }} = \int_{-\kappa T}^{\kappa \omega_c}
  \frac{d\omega^{\prime }}{2\pi} \frac{\gamma(\omega^{\prime })-
    \gamma(\omega)}{\omega - \omega^{\prime }} + \frac
  {\gamma(\omega)}{ 2 \pi} \cP \int_{-\kappa T}^{\kappa \omega_c} \frac 1 {\omega-\omega'} d \omega' \;.
\end{align}
The second term is
\begin{align}
  \frac  {\gamma(\omega)}{ 2 \pi} \cP \int_{-\kappa T}^{\kappa \omega_c} \frac 1 {\omega-\omega'} d \omega' = - \frac  {\gamma(\omega)}{ 2 \pi} \log\(\frac {\kappa \omega_c-\omega}{\kappa T-\omega}\)\;.
\end{align}

\begin{figure}[h]
  \centering
  \includegraphics[width=0.5 \textwidth]{lamb_shift_dominant}
  \caption{Dominant contribution to the Lamb shift $S(\omega)$. The blue line is $-(\gamma(\omega^{\prime })-
    \gamma(\omega))/(\omega - \omega^{\prime })$. The red line is $e^{\omega'/\omega_c}$.}
  \label{fig:lamb_shift_dominant}
\end{figure}
The first term does not have a singularity anymore. For an Ohmic spectral density $\gamma(\omega) \propto \eta \omega e^{-\omega/\omega_c}$, and $\omega_c \gg T, \omega$, the dominant contribution to the first term comes from the high frequency range. Setting $T, \omega \rightarrow 0$ this term can be approximated as
\begin{align}
  \frac{\gamma(\omega^{\prime })-
    \gamma(\omega)}{\omega - \omega^{\prime }} \rightarrow e^{-\omega'/\omega_c}\;,
\end{align}
which gives
\begin{align}
   \int_{-\kappa T}^{\kappa \omega_c}
  \frac{d\omega^{\prime }}{2\pi} \frac{\gamma(\omega^{\prime })-
    \gamma(\omega)}{\omega - \omega^{\prime }} \approx -\eta \int_0^\infty \frac{d \omega'}{2 \pi} e^{-\omega'/\omega_c} = -\frac{\eta}{2 \pi} \omega_c\;.
\end{align}
Therefore
\begin{align}
  S(\omega) \approx -\frac \eta {2 \pi} \( \omega_c + \omega \log(\omega_c/T)\)\;.
\end{align}

This is problematic
because the high-frequency cutoff is a big parameter (of unclear
physical meaning and difficult to measure in our context), and therefore the Lamb shift will
dominate the Redfield equation dynamics.

One solution is to do an adiabatic renormalization of each single qubit tunneling energy $\Delta$ tracing over the high frequency modes of the corresponding bath (see~\cite{leggett1987dynamics} and the technique due to Mark Dykman in appendix~\ref{app:tunneling_renormalization}). This approximation traces over bath modes with frequencies $\omega_Q >> T, E_{\rm max}$, where $E_{\rm max}$ is the highest system energy. The price we pay is that the single qubit tunneling energy gets renormalized
\begin{align}
  \Delta \longrightarrow \Delta_r = \Delta\cdot f(\omega_Q, \eta, \omega_c)\;.
\end{align}
Nevertheless, the measured single qubit parameters are fitted to experimental data obtained in the presence of the bath. That is, the measured energy is the renormalized $\Delta_r$, not the naked $\Delta$. Note that for independent baths the renormalization is done for each independent qubit bath, and the quantum master equation obtained is consistent with the measured qubits values. With this mind, the Lamb shift in the quantum master equation has a value
\begin{align}
  S_e(\omega) \approx - \frac{\eta \omega_Q}{2 \pi}\;.
\end{align}

As we noted above, the Lamb shift only affects the dynamical evolution of the phases of the density state in the instantaneous eigenbasis. Therefore, it can be seen as a small perturbation to the system Hamiltonian, which we can {\rm ignore}, as long as
\begin{align}\label{eq:lamb_shift_bound}
  \textrm{ system gap} \gg \frac {\eta T}{2 \pi}\;.
\end{align}

\subsubsection{D-Wave's decoherence parameters}
The dominant system-bath coupling for flux qubits is due to flux
fluctuations in the body of the qubit, and can be written as
\begin{align}
  H_I = \hat I_p \delta \Phi_B\;,
\end{align}
where $\hat I_p$ is the persistent current operator of the qubit~\cite{johnson2011quantum}. It has been found experimentally that an Ohmic spectral density
matches well the spectrum of the effective correlation functions $\avg{\delta \Phi_B(\tau) \delta \Phi_B(0)}$ of the bath in D-Wave's processor in the high
frequency spectrum relevant for the dynamical master
equation~\cite{PhysRevB.83.180502}. The bath coupling parameter $\eta$ is measured fitting the tail of the microscopic resonant tunneling rate (MRT) in the incoherent qubit regime $I_p(1) \Phi_B \gg \Delta$, where $\Delta$ is the qubit tunneling energy. The notation $I_p(1)$ signifies that this is the persistent current at the end of quantum annealing trajectory with $I_p(s)$ defined for $s \in [0,1]$. 

Restricting in the usual way to the lowest eigenstates of the system flux qubit we write $\hat I_p = I_p \sigma_z$. Because the coupling parameter $\eta$ is measured in the incoherent regime with persistent current $I_p(1)$ we can define a dimensionless bath coupling operator 
\begin{align}
  A_j(s) = \frac{I_p(s) }{ I_p(1)} \sigma^z\;.
\end{align}
 Incorporating the factor $I_p(s) / I_p(1)$ in the expression for the
 bath spectral density we write
\begin{align}
  \gamma_{j\beta}(\omega)  &= \frac{\eta\,\hbar \omega}{1 - e^{-\beta|
      \omega|}} \frac {I_p(s)^2}{I_p(1)^2} \left(
    \theta(\omega)+ e^{-\beta |\omega|} \theta(-\omega) \right)\delta_{j\beta}\;,
\end{align}
where we have used a bath high frequency renormalization cutoff $\omega_Q >> \omega$. We include Planck's constant $\hbar$ explicitly to fix the energy units. The coupling parameter for the Vesuvius chip we use is measured to be $\eta \approx 0.06$. The temperature is $T \approx 15$ mK. At the phase transition point of interest during quantum annealing for the current D-Wave annealing schedule we obtain the ratio $I_p(s)^2/I_p(1)^2 \approx 1/3$.

The fast bath approximation using when deriving the Redfield equation depends on the
bath time-scale $\tau_B$. An Ohmic bath has a bath correlation
time-scale of order $1/T$. Note that this equation
is derived in the interaction picture, and the only time scales of
interest $\tau_R$ and $\tau_B$, not the time scale of the Bohr
frequencies of the system. From the condition $\tau_R >> \tau_B$ we need
\begin{align}
  \nu \ll \frac 3 \eta \frac {k_B T} {h}\;,
\end{align}
which is a good approximation in our case, given the small value of $\eta$ (explicitly, this is $\nu \ll 15$ GHz, in units of cycles per second). 

We also ignore the Lamb shift term up to very small gaps. From Eq.~\eqref{eq:lamb_shift_bound}, and including the factor $I_p(s)^2/I_p(1)^2 \approx 1/3$
\begin{align}
  \nu \gg \frac \eta 3 \frac {k_B T} {h}\;.
\end{align}
Explicitly, this is $\nu \gg 1$ MHz (with energy in units of cycles per second).

\section{Tunneling dissipative renormalization}\label{app:tunneling_renormalization}

We study a single qubit coupled with a $\sigma^z$ coupling to a bosonic bath
\begin{align}
  H = \frac 1 2 (\epsilon \sigma^z + \Delta \sigma^x )+ \sigma^z\sum_q u_q(b_q+b_q^\dagger) + \sum_q \omega_q b_q^\dagger b_q\;.
\end{align}
We can apply the results here to a multiqubit system with independent bosonic baths. The goal is to trace over very fast high frequency vacuum modes in the environment, which will result in a renormalization of the tunneling energy (see, for instance, Sec. III.C. in~\cite{leggett1987dynamics}).

\subsection{Hamiltonian transformation}
We define the unitary
\begin{align}
  U = e^{ \sum_q \frac {u_q} {\omega_q} (b_q-b_q^\dagger) \sigma^z}\;.
\end{align}
It is easy to check that indeed $U U^\dagger = 1$. 
We are interested in the transformed Hamiltonian
\begin{align}
  \tilde H = U^\dagger H U\;.
\end{align}

Define 
\begin{align}
  \cO = -\sum_q \frac {u_q} {\omega_q} (b_q-b_q^\dagger) \sigma^z\;.
\end{align}
We have
\begin{align}
 U^\dagger H U = e^{\cO} H e^{-\cO} = e^{\rad(\cO)} H\;,
\end{align}
where
\begin{align}
  \rad(\cO)(H) = [\cO,H]\;.
\end{align}

We start with the transformation of the operator
\begin{align}
  \tilde b_q^\dagger = U^\dagger b_q^\dagger U\;.
\end{align}
We have
\begin{align}
  [\cO, b_q^\dagger] = \sum_{q'} \frac {u_{q'}} {\omega_{q'}} [b_{q'}^\dagger, b_q] \sigma^z = - \frac {u_q} {\omega_q} \sigma^z\;,
\end{align}
and
\begin{align}
 [\cO, [\cO, b_q^\dagger] ] = 0\;.
\end{align}
Therefore
\begin{align}
  b_q^\dagger = b_q^\dagger - \frac {u_q} {\omega_q} \sigma^z\;.
\end{align}
Now we do the transformation of $\sigma^+$. We have
\begin{align}
  [\cO, \sigma^+] = -\sum_q \frac {u_q} {\omega_q} (b_q-b_q^\dagger) [\sigma^z, \sigma^+] = -\sum_q \frac {u_q} {\omega_q} (b_q-b_q^\dagger) 2 \sigma^+\;.
\end{align}
Therefore
\begin{align}
  \tilde \sigma^+ = e^{ - 2 \sum_q \frac {u_q} {\omega_q} (b_q-b_q^\dagger)} \sigma^+\;.
\end{align}
We then obtain
\begin{align}
  2 \tilde \sigma^x = e^{- 2 \sum_q \frac {u_q} {\omega_q} (b_q-b_q^\dagger)} \sigma^+ + e^{ 2 \sum_q \frac {u_q} {\omega_q} (b_q-b_q^\dagger)} \sigma^-\;.
\end{align}

Putting it all together, we get the transformation
\begin{align}
  \tilde H  & = \frac \epsilon 2 \sigma^z + \frac \Delta 4 \(e^{- 2 \sum_q \frac {u_q} {\omega_q} (b_q-b_q^\dagger)} \sigma^+  + e^{ 2 \sum_q \frac {u_q} {\omega_q} (b_q-b_q^\dagger)} \sigma^-\) \\
  &\quad+ \sigma^z\sum_q u_q(b_q+b_q^\dagger) - 2 \sum_q \frac {u_q^2}
  {\omega_q}  
  \\
  &\quad+ \sum_q \omega_q b_q^\dagger b_q -\sigma^z\sum_q u_q b_q^\dagger
  -\sigma^z \sum_q u_q b_q + \sum_q \frac {u_q^2}{\omega_q} \\
  & =\frac \epsilon 2 \sigma^z + \frac \Delta 4 \(e^{- 2 \sum_q \frac {u_q} {\omega_q} (b_q-b_q^\dagger)} \sigma^+  + e^{ 2 \sum_q \frac {u_q} {\omega_q} (b_q-b_q^\dagger)} \sigma^-\) \\
  &\quad + \sum_q \omega_q b_q^\dagger b_q -  \sum_q \frac {u_q^2}{\omega_q} 
\end{align}

\subsection{Tunneling renormalization}
We can do the same transformation but summing only high frequency bath
modes above a threshold $Q$. That is, we use the transformation
\begin{align}
    U' = e^{ \sum_{q>Q} \frac {u_q} {\omega_q} (b_q-b_q^\dagger) \sigma^z}
\end{align}
We chose $Q$ such that $\omega_Q \gg T, E_{\rm max}$, where $E_{\rm max}$ is a bound on the highest energy populated system state (in the single qubit case, $E_{\rm max} = \epsilon$, in a multiqubit system  it will depend on the system dynamics). Then the bath state of all the modes in the sum
is the vacuum. 

We want to study the dynamics tracing over the bath high-frequency modes
\begin{align}
  \i \TrBQ \frac {\partial \;\rho_S \otimes \rho_B} {\partial t} &= \TrBQ [H, \rho_S \otimes \rho_B]  \\
  &= \TrBQ [\tilde H, U' \rho_S \otimes \rho_B U'^\dagger]\;.
\end{align}

First consider the state $U'\rho_S \otimes \rho_B U'^\dagger$. The operator $U$ is a displacement $D(\pm \sum_{q>Q} \frac {u_q} {\omega_q})$ of the bath vacuum state conditional on the state of the system in the $\sigma^z$ basis. This are high frequency modes, much faster than the time-scale of all the dynamics that we are interested in, and they will relax to their vacuum state. We approximate
\begin{align}
  U' \rho_S \otimes \rho_B U'^\dagger \rightarrow \rho_S \otimes \rho_B\;.
\end{align}

We need to calculate to calculate expectation values of displacement operators over the vacuum.
Using $e^{A+B} = e^A  e^{[A,B]/2} e^B$, we first note that
\begin{align}
    e^{ 2 \sum_{q>Q} \frac {u_q} {\omega_q} (b_q-b_q^\dagger)}  &=
    e^{- 2 \sum_{q>Q} \frac {u_q} {\omega_q} b_q^\dagger} e^{ 2
      \sum_{q>Q} \frac {u_q} {\omega_q} b_q} e^{ 2 \sum_{q>Q} \frac
      {u_q^2} {\omega_q^2} }     \\
    e^{ -2 \sum_{q>Q} \frac {u_q} {\omega_q} (b_q-b_q^\dagger)}  &= e^{ 2 \sum_{q>Q} \frac {u_q} {\omega_q} b_q^\dagger} e^{ -2 \sum_{q>Q} \frac {u_q} {\omega_q} b_q} e^{ 2 \sum_{q>Q} \frac {u_q^2} {\omega_q^2} }\;.
  \end{align}

When taking expectation values we note that
\begin{align}
    \bra {{\rm vac}_q} e^{ \xi_1 b_q^\dagger} e^{ \xi_2 b_q} \ket {{\rm vac}_q} = 1\;.
\end{align}
Therefore, when tracing over the bath high frequency modes the contribution of the displacement operators is
  $\exp\( 2 \sum_{q>Q} \frac {u_q^2} {\omega_q^2}\)$.
Putting this into the expression for $\tilde H$ we obtain the renormalized Hamiltonian (up to a constant factor)
\begin{align}
H_r =  \frac \epsilon 2 \sigma^z + \frac \Delta 2 e^{2 \sum_{q>Q} \frac {u_q^2} {\omega_q^2}} \sigma^x  + \sum_q \omega_q b_q^\dagger b_q \;.
\end{align}

In conclusion, the net result of the transformation and tracing over high frequency modes is a renormalization of the tunneling energy to
\begin{align}
  \Delta_r = \Delta e^{2 \sum_{q>Q} \frac {u_q^2} {\omega_q^2}} \;.
\end{align}
{\bf If the tunneling energy is measured experimentally in the presence of the bath, then the measured valued is already $\Delta_r$}, not the naked $\Delta$. 

\subsection{Estimate of the renormalization factor}
We can estimate the value of the renormalization factor $e^{2 \sum_{q>Q} \frac {u_q^2} {\omega_q^2}}$ for an Ohmic
spectral density
\begin{align}
  \sum_{q>Q} u_q = \int_{w_Q}^\infty d\omega \frac{J(\omega)}{2 \pi} =
  \int_{w_Q}^\infty d\omega \frac{\eta \omega e^{-\omega/\omega_c}}{2 \pi} \;.
\end{align}
We obtain
\begin{align}
    \sum_{q>Q} \frac {u_q^2} {\omega_q^2}=
  \frac{\eta^2}{4\pi^2}\int_{w_Q}^\infty d\omega e^{-2\omega/\omega_c}
  = -\frac{\eta^2}{4\pi^2} \frac {\omega_c} 2\( 1 - e^{-2 \omega_Q/\omega_c}\)\;.
\end{align}
Therefore
\begin{align}
    e^{2 \sum_{q>Q} \frac {u_q^2} {\omega_q^2}} = \exp\(\frac{\eta^2
      \omega_c}{4\pi^2} \(  e^{-2 \omega_Q/\omega_c} - 1\)\)\;.
\end{align}

\section{Reorganization energy in the coherent regime}

Reference~\cite{amin2009non} Sec. IV.C solves the reorganization energy for a representative spectral density. For a resonance time scale $\Delta \ll \omega_\lf$ the reorganization energy is consistent with the one reproduced in the previous section. On the other hand, in the coherent regime $\omega \gg \omega_\lf$, the corresponding reorganization energy disappears $\epsilon_p(\Delta) \rightarrow 0$. The reason is that $1/\omega_\lf$ corresponds to the response time of the low frequency bath, and at faster time-scales the bath does not have time to adapt. 

\subsection{D-Wave's low frequency noise parameters}

Similarly to the high frequency bath coupling, the dominant system-bath coupling for flux qubits is due to flux
fluctuations in the body of the qubit, and can be written as
\begin{align}
  H_I = \hat I_p \delta \Phi_B\;,
\end{align}
where $\hat I_p$ is the persistent current operator of the qubit~\cite{johnson2011quantum}. Because the noise is probed in the incoherent regime with persistent current $I_p(1)$, the factor $I_p(s) / I_p(1)$ must be incorporated in the expression for the low frequency bath spectral density
\begin{align}
  \gamma_\lf(\omega,s ) = \frac {I_p(s)^2 }{ I_p(1)^2 } \gamma_\lf  \;.
\end{align}
Correspondingly, because $W^2$ scales linearly with the spectral function, the low frequency resonance width scales like
\begin{align}
  W(s) = \frac {I_p(s)}{ I_p(1)} W(1)\;.
\end{align}

At the phase transition point of interest during quantum annealing for the current D-Wave annealing schedule we obtain the ratio $I_p(s)/I_p(0) \approx 0.6$. The value of $W(1)$ has been measured experimentally by D-Wave with the technique in Ref.~\cite{PhysRevB.83.180502} to be $W(1) \approx 0.22$ GHz. Therefore, at the phase transition $W \approx 0.13$ GHz. 

One consequence is that given the assumption $\omega_\lf << W$ in the derivation of the Gaussian noise, and the comment above about the reorganization energy in the coherent regime, {\bf the reorganization energy can be ignored for $\Delta \gg 0.13$ GHz}.
